# Supplementary material for: EntSUM: A Data Set for Entity-Centric Summarization
Source: arXiv:2204.02213 source file (2022-04-05)
Supplement: Supplementary file 1 [file appendix.tex]

% % We tried the following 3 methods to group entities in step 1 with different surface names.  To test each method, we manually inspected 54 salient entities and their extracted groups from 10 random documents (salient entities were marked by the annotators). We ended up using substring matching which reduced entities (with saliency > 1.5) after step 1 from 3866 to 2788.

% % Method Entities after grouping Errors Duplicates
% % Substring Matching 39 (72%) 1 2
% % SpanBERT (Group entities belonging to the same coreference cluster. Used substring matching to check if an entity is in a cluster as exact matching was giving very less matches.) 31 (57%) 10 0
% % Sieve Coref (similar to SpanBERT) 42 (77%) 12  1

% % Coreference Resolution with SpanBERT did not group entities properly because the surface name of the entities looked very different from the names in the clusters.

% OLD SUMMARY STATISTICS

% \begin{table}
%     \small
%     \centering
%     \begin{tabular}{l|cc|cc}
%     \hline
%     & \multicolumn{2}{c|}{\textbf{\textsc{ExSUM$_{ONE}$}}} &  \multicolumn{2}{c}{\textbf{\textsc{ExSUM$_{TWO}$}}} \\
%     & \textbf{Med.} & \textbf{
%     High} &  \textbf{Med.} & \textbf{High} \\
%     \hline
%     \# of entities & 1456 & 465 & 644 & 223 \\
%     \hline
%     \multicolumn{5}{l}{\textit{\textbf{Average Stats (per article)}}} \\
%     \hline
%     \# of premarked sents.  & 3.19 & 5.34 & 3.73 & 6.35 \\
%     \# of salient sents.  & 4.67 & 8.24 & 5.57 & 9.26\\
%     \# of summary sents.  & 2.33 & 2.63 & 2.58 & 2.73 \\
%     summary word len. & 78.6 & 87.9 & 81.5 & 88.7\\
%     summary char. len. & 427.7 & 481.9 & 441.7 & 485.1 \\
%     \hline 
%     \end{tabular}
%   \caption{\textsc{ExSUM} statistics with respect to entity salience. \textbf{Med.} and \textbf{High} refer to entity salience values between $1-2$ and $2-3$ respectively.}
%   \label{table:salience_stats}
% \end{table}


% % ENTITY SALIENT SENTENCES GOLD STATS

% % 4 documents, 34 entities, 819 sentences.
% % Collected 3 annotations for each HIT.
% % 4 annotators in total (Mounica, Mayank, Daniel, Chuck).
% % IAA - Binary Alpha: 0.640
% % The 3 annotators completely agreed on 702 sentences out of  819 sentences (86%).
% % There were majorly 3 types disagreements: 
% % Context for a salient sentences was not marked. 
% % Opinions and speculations marked as salient (Opinions are tricky. Most of the direct quotes seem like they are opinions)
% % Split sentences are not marked.
% % Decided to go with only salient entities.

% % Number of annotations: 8364
% % Binary Krippendorf's Alpha: 0.744
% % Number of entities:  2788
% % Number of documents:  645
% % \% of sentences where all the annotators agreed,  84844 95894 88.4
% % Number of pre-marked sentences:  10945
% % Avg. number of pre-marked sentences:  3.95
% % Number of salient sentences (after adjudication):  16280
% % Avg. number of salient sentences (after adjudication):  5.8
% % Number of pre-marked salient sentences:  10752
% % Avg. number of pre-marked salient sentences:  3.85
% % Number of sentences:  95894
% % Avg. number of sentences:  34.39

% % ENTITY SUMMARY GOLD STATS

% % Number of entities:  15
% % Number of documents:  3
% % Annotators: Mayank and Mounica

% % All sentences:
% % Binary Krippendorf's Alpha: 0.844
% % % of sentences where all the annotators agreed,  
% % 586 599 98.2%

% % Salient sentences only:
% % Binary Krippendorf's Alpha: 0.683
% % % of sentences where all the annotators agreed,  
% % 51 62 85.4%

% % Number of entities:  2788
% % Number of annotations: 3655
% % Binary Krippendorf's Alpha (only salient sentences): 0.539

% % Average Summary Word Length:  72.34
% % Average Summary Character Length:  438.32
% % Average Number of selected sentences:  2.4

% % Number of salient sentences:  21931
% % Number of salient sentences selected for summary:  8922

% % \begin{table*}
% %     \small
% %     \centering
% %     \begin{tabular}{l|cc|cc||cc|cc}
% %     \hline
% %     \textbf{Average Stats}& \multicolumn{2}{c|}{\textbf{\textsc{ExSUM$_{ONE}$}}} &  \multicolumn{2}{c||}{\textbf{\textsc{ExSUM$_{TWO}$}}} & \multicolumn{2}{c|}{\textbf{\textsc{ExSUM$_{ONE}$}}} &  \multicolumn{2}{c}{\textbf{\textsc{ExSUM$_{TWO}$}}} \\
% %     & \textbf{PER} & \textbf{ORG} &  \textbf{PER} & \textbf{ORG} & \textbf{Med.} & \textbf{
% %     High} &  \textbf{Med.} & \textbf{High} \\
% %     \hline
% %     \# of entities & 1175 & 746 & 566 & 301  & 1456 & 465 & 644 & 223 \\
% %     \hline
% %     \multicolumn{5}{l}{\textit{\textbf{Average Stats (per article)}}} \\
% %     \hline
% %     \# of premarked sents.  & 4.03 & 3.21  & 4.61  & 4.01 & 3.19 & 5.34 & 3.73 & 6.35 \\
% %     \# of salient sents.  & 6.06 & 4.71  & 6.95 & 5.7  & 4.67 & 8.24 & 5.57 & 9.26 \\
% %     \# of summary sents.  & 2.52 & 2.22 & 2.73 & 2.4 & 2.33 & 2.63 & 2.58 & 2.73 \\
% %     summary word len. & 84.2 &  75.6 & 86.6 & 77.3 & 78.6 & 87.9 & 81.5 & 88.7 \\
% %     summary char. len. & 454.3 & 419.3 & 466.6 & 426.9 & 427.7 & 481.9 & 441.7 & 485.1 \\
% %     \hline 
% %     \end{tabular}
% %   \caption{\textsc{ExSUM} statistics with respect to entity type and salience. \textbf{PER} and \textbf{ORG} refer to ``Person'' and ``Organization'' entity types respectively. \textbf{Med.} and \textbf{High} refer to entity salience values between $1-2$ and $2-3$ respectively.}
% %   \label{table:type_stats}
% % \end{table*}

% % Overall vs Entity-centric stats
% % % One Annotation
% % % #instances
% % % % novel unigram / bigram
% % % Length Stats (S/W/C)
% % % Avg. number of pre-marked/salient/summary sentences
% % % Compression ratio
% % % Overall NYT summaries

% % % 41265
% % % 11.4 / 39.5
% % % 4.87 / 116.96 / 677.48

% % % SRC: 36.9 / 1021.1 / 5471

% % % -
% % % 0.117
% % % NYT centric-summaries

% % % 1921
% % % 0.61 / 4.95
% % % 2.4 / 80.9 / 440.8

% % % SRC: 34.7 / 1014 / 5379

% % % 3.71 / 5.53 / 2.34

% % % Wrt salient:
% % % 0.64

% % % Wrt source:
% % % 0.0928
% % % Overall CNN DailyMail
% % % 312085
% % % 13.3 / 49.95
% % % 3.67 / 56.38 / 297.15

% % % SRC:  33.1/ 782.2/ 3998.8
% % % -
% % % 0.089

% % % Two Annotations
  
% % % #instances
% % % % novel unigram / bigram
% % % Length Stats (S/W/C)
% % % Avg. number of pre-marked/salient/summary sentences
% % % Compression ratio
% % % Overall NYT summaries

% % % 41265
% % % 11.4 / 39.5
% % % 4.87 / 116.96 / 677.48

% % % SRC: 36.9 / 1021.1 / 5471

% % % -
% % % 0.117
% % % NYT centric-summaries

% % % 1734
% % % 1.3 / 8.09
% % % 2.6 / 83.3 / 452.8

% % % SRC: 33.7 / 977 / 5189
% % % 4.4 / 6.52 / 2.56

% % % Wrt salient:
% % % 0.58

% % % Wrt source:
% % % 0.0935
% % % Overall CNN DailyMail
% % % 312085
% % % 13.3 / 49.95
% % % 3.67 / 56.38 / 297.15

% % % SRC:  33.1/ 782.2/ 3998.8
% % % -
% % % 0.089


% % \subsubsection{Length Statistics for entity salience}
% % One Annotation

% %  Entity Salience for NYT Entity-centric summaries 
% % (first batch of 701 tasks - 2 annotations for each task)
% % #annotations
% % Length Stats (S/W/C)
% % Avg. number of pre-marked/salient/summary sentences
% % 1 - 2


% % 1456
% %  2.33 / 78.63 / 427.67


% % 3.19 / 4.67 / 2.28
% % 2 - 3
% % 465
% % 2.63 / 87.86 / 481.89



% % 5.34 / 8.24 / 2.5


% % Two Annotations
% %  Entity Salience for NYT Entity-centric summaries 
% % (first batch of 701 tasks - 2 annotations for each task)
% % #annotations
% % Length Stats (S/W/C)
% % Avg. number of pre-marked/salient/summary sentences
% % 1 - 2


% % 1288
% %  2.58 / 81.52 / 441.74


% % 3.73 / 5.57 / 2.51
% % 2 - 3
% % 446
% % 2.73 / 88.69 / 485.06



% % 6.35 / 9.26 / 2.71


% % \subsubsection{Length Statistics for each entity type}
% % One Annotation
% %  Entity Type for NYT Entity-centric summaries 
% % (first batch of 701 tasks - 2 annotations for each task)
% % #annotations
% % Length Stats (S/W/C)
% % Avg. number of pre-marked/salient/summary sentences
% % Person


% % 1175
% %  2.52 / 84.2 / 454.3


% % 4.03 / 6.06 / 2.44
% % Organization
% % 746
% % 2.22 / 75.6 / 419.3


% % 3.21 / 4.71 / 2.17

% % Two Annotations
% %  Entity Type for NYT Entity-centric summaries 
% % (first batch of 701 tasks - 2 annotations for each task)
% % #annotations
% % Length Stats (S/W/C)
% % Avg. number of pre-marked/salient/summary sentences
% % Person


% % 1132
% %  2.73 / 86.61 / 466.68


% % 4.61 / 6.95 / 2.66
% % Organization
% % 602
% % 2.4 / 77.26 / 426.94


% % 4.01 / 5.7 / 2.36

% \section{Results Dump}
% \begin{table}[]
% \begin{tabular}{lll}
%                               & \begin{tabular}[c]{@{}l@{}}F1 (salient)\\ Adjudicated\end{tabular} & F1 (summary) \\
% Lead3 overall                  & 15.8                                                               & 17.9         \\
% Lead 3 - entity (string match) & 39.4                                                               & 67.1         \\
% Lead 3 - entity (coref)        & 50.0                                                               & 69.2         \\
% Lead3 - salient oracle         & 61.5                                                               & 79.4         \\
% Lead 3 - summary oracle        & 57.7                                                               & 97.7        
% \end{tabular}
% \caption{One annotation dataset}
% \end{table}

% \begin{table}[]
% \begin{tabular}{llll}
%                               & \begin{tabular}[c]{@{}l@{}}F1 (salient)\\ Adjudicated\end{tabular} & \begin{tabular}[c]{@{}l@{}}F1 (summary)\\ Max of 2 annotations\end{tabular} & \begin{tabular}[c]{@{}l@{}}F1 (summary)\\ Average of 2 annotations\end{tabular} \\
% Lead3 overall                  & 15.7                                                               & 20.8                                                                        & 18.1                                                                            \\
% Lead 3 - entity (string match) & 39.2                                                               & 67.9                                                                        & 61.4                                                                            \\
% Lead 3 - entity (coref)        & 47.5                                                               & 74.4                                                                        & 67.2                                                                            \\
% Lead3 - salient oracle         & 56.5                                                               & 83.0                                                                        & 75.2                                                                            \\
% Lead 3 - summary oracle        & 52.7                                                               & 96.5                                                                        & 85.5                                                                           
% \end{tabular}
% \caption{Two annotation dataset}
% \end{table}

% \begin{table*}[]
% \begin{tabular}{llllll}
% Baselines                                                                                              & R1   & R2   & RL   & BERTScore & Len (S/W/C)  \\
% Lead 3 - overall                                                                                       & 35.4 & 20.2 & 31.9 & 57.6      & 3/100/549    \\
% BERTSUM-overall (CNNDailyMail)                                                                         & 34.3 & 18.0 & 30.5 & 56.9      & 3/97/534     \\
% BERTSUM-overall (NYT)                                                                                  & 34.8 & 19.0 & 31.2 & 57.8      & 3/110/609    \\
% BERTSUM - entity (NYT - trained with top 3 sentences -  generated top 3)                               & 32.5 & 15.9 & 28.5 & 55.6      & 3/98/527     \\
% BERTSUM - entity (NYT - trained with all salient sentences in the reference - generated top 3)         & 33.6 & 17.2 & 29.5 & 56.3      & 3/97/524     \\
% BERTSUM - entity (NYT - trained with all salient sentences in the reference - generated top 6)         & 33.2 & 19.1 & 30.2 & 57.9      & 6.2/187/1014 \\
% SPANBERT\_COREF - entity (NYT - trained with all salient sentences in the reference - generated top 3) & 35.9 & 20.6 & 32.3 & 58.9      & 3.2/105/568  \\
% Lead 3 - entity                                                                                        & 71.3 & 64.3 & 68.2 & 79.4      & 2.7/92/497   \\
% Lead 3 -  salient oracle                                                                               & 79.4 & 74.1 & 76.4 & 84.8      & 2.7/91/488   \\
% Lead 3 - summary oracle                                                                                & 91.0 & 87.8 & 88.4 & 91.6      & 2.5/86/467 \\
% BERTSUM - entity (CNN - trained with all salient sentences in the reference - generated top 3)         & 31.7 & 15.0 & 27.8 & 55.2 & 3.2/93/504  \\
% BERTSUM - entity (CNN - trained with all salient sentences in the reference - generated top 6)         & 32.2 & 17.3 & 29.1 & 57.0 & 6.2/182/994 \\
% SPANBERT\_COREF - entity (CNN - trained with all salient sentences in the reference - generated top 3) & 32.8 & 16.1 & 28.8 & 55.9 & 3.2/98/531 
% \end{tabular}
% \caption{One annotation dataset}
% \end{table*}



% \begin{table*}[]
% \begin{tabular}{lll}
% Baselines                                                                                              & F1 (salient) Adjudicated & F1 (summary) \\
% Lead3 overall                                                                                          & 15.8                     & 17.9         \\
% BERTSUM-overall (CNNDailyMail)                                                                         & 15.0                     & 15.4         \\
% BERTSUM-overall (NYT)                                                                                  & 15.4                     & 16.3         \\
% BERTSUM - entity (NYT - trained with top 3 salient sentences** in the reference - generated top 3 )    & 15.3                     & 13.5         \\
% BERTSUM - entity (NYT - trained with all salient sentences in the reference - generated top 3)         & 16.2                     & 14.8         \\
% BERTSUM - entity (NYT - trained with all salient sentences in the reference - generated top 6)         & 21.7                     & 16.4         \\
% SPANBERT\_COREF - entity (NYT - trained with all salient sentences in the reference - generated top 3) & 18.9                     & 18.6         \\
% Lead3 entity                                                                                           & 50.0                     & 69.2         \\
% Lead3 - salient oracle                                                                                 & 61.5                     & 79.4         \\
% Lead 3 - summary oracle                                                                                & 57.7                     & 97.7    \\
% BERTSUM - entity (CNN - trained with all salient sentences in the reference - generated top 3)         & 15.4 & 12.6 \\
% BERTSUM - entity (CNN - trained with all salient sentences in the reference - generated top 6)         & 21.2 & 14.3 \\
% SPANBERT\_COREF - entity (CNN - trained with all salient sentences in the reference - generated top 3) & 15.6 & 13.6
% \end{tabular}
% \caption{One annotation dataset}
% \end{table*}

% \begin{table*}[]
% \begin{tabular}{llllll}
% Baselines (tested on 700 instances)                                                                    & R1   & R2   & RL   & BERTScore & Len (S/W/C) \\
% Lead 3 - overall                                                                                       & 32.3 & 16.8 & 28.9 & 59.9      & 3/98/538    \\
% BERTSUM-overall (CNNDailyMail)                                                                         & 31.6 & 15.4 & 28.0 & 59.4      & 3/97/535    \\
% BERTSUM-overall (NYT)                                                                                  & 31.6 & 15.1 & 27.9 & 59.2      & 3.1/110/604 \\
% BERTSUM - entity (NYT - trained with top 3 sentences -  generated top 3)                               & 29.7 & 12.3 & 25.6 & 57.8      & 3.2/97/528  \\
% BERTSUM - entity (NYT - trained with all salient sentences in the reference - generated top 3)         & 31.0 & 14.6 & 27.3 & 58.8      & 3.1/96/523  \\
% BERTSUM - entity (NYT - trained with all salient sentences in the reference - generated top 6)         & 31.1 & 16.6 & 28.2 & 60.1      & 6/182/989   \\
% SPANBERT\_COREF - entity (NYT - trained with all salient sentences in the reference - generated top 3) & 33.4 & 17.3 & 29.6 & 60.6      & 3.3/104/562 \\
% Lead 3 - entity                                                                                        & 67.4 & 58.6 & 63.5 & 85.9      & 2.8/92/496  \\
% Lead 3 -  salient oracle                                                                               & 72.4 & 64.3 & 68.5 & 91.2      & 2.6/86/465  \\
% Lead 3 - summary oracle                                                                                & 62.0 & 52.1 & 58.0 & 81.6      & 2.9/93/504 \\
% BERTSUM - entity (CNN - trained with all salient sentences in the reference - generated top 3)         & 29.3 & 12.0 & 25.2 & 57.1 & 3.3/94/509   \\
% BERTSUM - entity (CNN - trained with all salient sentences in the reference - generated top 6)         & 29.7 & 14.4 & 26.6 & 59.0 & 6.4/187/1008 \\
% SPANBERT\_COREF - entity (CNN - trained with all salient sentences in the reference - generated top 3) & 30.0 & 13.1 & 26.1 & 58.3 & 3.1/93/507  
% \end{tabular}
% \caption{Two annotations dataset}
% \end{table*}


% \begin{table*}[]
% \begin{tabular}{llllll}
% \multicolumn{1}{l}{}                                         & \multicolumn{1}{l}{ROUGE-1}                      & \multicolumn{1}{l}{ROUGE-2} & \multicolumn{1}{l}{ROUGE-L} & \multicolumn{1}{l}{BERTScore} & Len (S/W/C) \\ 
% \multicolumn{1}{l}{Lead 3 - overall} & \multicolumn{1}{l}{35.4}                         & \multicolumn{1}{l}{20.2}    & \multicolumn{1}{l}{31.9}    & \multicolumn{1}{l}{57.6}      & 3/100/549   \\ 
% \multicolumn{1}{l}{Lead 3 - entity (string match)}           & \multicolumn{1}{l}{66.8} & \multicolumn{1}{l}{62.3}    & \multicolumn{1}{l}{63.8}    & \multicolumn{1}{l}{78.3}      & 1.6/55/302  \\ 
% \multicolumn{1}{l}{Lead 3 - entity (coref)}                  & \multicolumn{1}{l}{71.3}                         & \multicolumn{1}{l}{64.3}    & \multicolumn{1}{l}{68.2}    & \multicolumn{1}{l}{79.4}      & 2.7/92/497  \\ 
% Lead 3 -  salient oracle               & 79.4                                              & 74.1                         & 76.4                         & 84.8                           & 2.7/91/488  \\
% Lead 3 - summary oracle                                        & 91.0                      & 87.8                         & 88.4                         & 91.6                           & 2.5/86/467  \\
% CTRL-Sum (CNNDailyMail)                                        & 29.5                                              & 19.4                         & 27.3                         & 59.5                           & 1.6/26/143  \\
% CTRL-Sum (NYT)                                                 & 33.5                                              & 18.7                         & 30.9                         & 57.6                           & 4.3/111/635 \\
% CTRL-Sum (NYT) - truncated 3                                   & 31.9                                              & 16.9                         & 29.1                         & 56.8                           & 2.9/86/487  \\
% Fan et. al (CNNDailyMail)                                      & 28.8                                              & 12.2                         & 25.1                         & 52.6                           & 2.6/50/280/ \\
% Fan et. al (NYT)                       & 29.6                                              & 14.3                         & 26.6                         & 54.1                           & 3.9/103/577 \\
% Fan et. al (NYT) - truncated 3                                 & 26.9                      & 11.5                         & 23.9                         & 56.1                           & 2.8/85/481 
% \end{tabular}
% \caption{One annotation dataset}
% \end{table*}

% \begin{table*}[]
% \begin{tabular}{llllll}
%                               & ROUGE-1                      & ROUGE-2 & ROUGE-L & BERTScore & Len (S/W/C) \\
% Lead 3 - overall               & 32.3                         & 16.8    & 28.9    & 59.9      & 3/98/538    \\
% Lead 3 - entity (string match) & 55.3 & 48.0    & 51.4    & 80.3      & 1.6/55/298  \\
% Lead 3 - entity (coref)        & 62.0                         & 52.1    & 58.0    & 81.6      & 2.9/93/504  \\
% Lead 3 -  salient oracle       & 67.4                         & 58.6    & 63.5    & 85.9      & 2.8/92/496  \\
% Lead 3 - summary oracle        & 72.4 & 64.3    & 68.5    & 91.2      & 2.6/86/465  \\
% CTRL-Sum (CNNDailyMail)        & 26.9                         & 17.1    & 24.8    & 62.3      & 1.6/25/140  \\
% CTRL-Sum (NYT)                 & 30.3                         & 15.1    & 27.6    & 59.1      & 4.4/110/622 \\
% CTRL-Sum (NYT) - truncated 3   & 28.7                         & 13.2    & 25.5    & 58.1      & 2.9/85/484  \\
% Fan et. al (CNNDailyMail)      & 27.3                         & 10.8    & 23.7    & 54.6      & 2.6/51/288  \\
% Fan et. al (NYT)               & 27.4                         & 11.8    & 24.2    & 56.1      & 4.0/100/564 \\
% Fan et. al (NYT) - truncated 3 &                              &         &         &           &            
% \end{tabular}
% \caption{Two annotations dataset}
% \end{table*}


% \begin{table*}[]
% \begin{tabular}{llllll}
% Baselines                       & R1   & R2   & RL   & BScore & Len (S/W/C) \\
% Lead 3 - overall                & 35.4 & 20.2 & 31.9 & 57.6   & 3/100/549   \\
% CTRL-Sum                        & 33.5 & 18.7 & 30.9 & 57.6   & 4.3/111/635 \\
% ConvNet                         & 29.6 & 14.3 & 26.6 & 54.1   & 3.9/103/577 \\
% Lead 3 - entity  (string match) & 66.8 & 62.3 & 63.8 & 78.3   & 1.6/55/302  \\
% Lead 3 - entity  (coref)        & 71.3 & 64.3 & 68.2 & 79.4   & 2.7/92/497  \\
% GSUM Pretrained (CNNDailyMail)  & 41.1 & 25.8 & 38.2 & 62.1   & 3.6/405/74  \\
% Setup 1 (NYT)                   & 53.2 & 42.6 & 50.4 & 69.3   & 3.6/111/605 \\
% Setup 2  (NYT)                  & 63.6 & 54.9 & 60.7 & 75.0   & 3.3/99/541  \\
% Setup 3 (NYT)                   & 30.1 & 14.8 & 27.3 & 55.4   & 4.1/117/677 \\
% Setup 4 (NYT)                   & 30.2 & 15.0 & 27.4 & 55.2   & 4.1/119/688 \\
% Setup 5 (NYT)                   & 30.3 & 14.9 & 27.4 & 55.5   & 4/120/690 \\
% Setup 1 (CNNDM)  & 59.1 & 49.6 & 56.0 & 72.8 & 3.4/104/563 \\
% Setup 2  (CNNDM) & 65.6 & 57.3 & 62.6 & 76.4 & 3.1/93/506  \\
% Setup 3 (CNNDM)  & 30.4 & 13.5 & 27.2 & 55.2 & 3.6/73/405  \\
% Setup 4 (CNNDM)  & 31.5 & 14.7 & 28.2 & 56.0 & 3.5/76/419  \\
% Setup 5 (CNNDM)  & 32.4 & 15.5 & 29.0 & 56.3 & 3.4/78/431 
% \end{tabular}
% \caption{One annotation - GSUM}
% \end{table*}

% \begin{table*}[]
% \begin{tabular}{llllll}
% Baselines                      & R1   & R2   & RL   & BScore & Len (S/W/C) \\
% Lead 3 - overall               & 32.3 & 16.8 & 28.9 & 59.9   & 3/98/538    \\
% CTRL-Sum                       & 30.3 & 15.1 & 27.6 & 59.1   & 4.4/110/622 \\
% ConvNet                        & 27.4 & 11.8 & 24.2 & 56.1   & 4.0/100/564 \\
% Lead3 - entity (string match)  & 55.3 & 48.0 & 51.4 & 80.3   & 1.6/55/298  \\
% Lead 3 - entity (coref)        & 62.0 & 52.1 & 58.0 & 81.6   & 2.9/93/504  \\
% GSUM Pretrained (CNNDailyMail) & 38.5 & 22.8 & 35.3 & 65.0   & 3.6/75/410  \\
% Setup 1 (NYT)                  & 48.4 & 35.8 & 45.1 & 71.9   & 3.7/111/603 \\
% Setup 2  (NYT)                 & 56.7 & 45.7 & 53.2 & 77.8   & 3.4/548/101 \\
% Setup 3 (NYT)                  & 27.2 & 11.8 & 24.5 & 57.1   & 4.2/116/666 \\
% Setup 4 (NYT)                  & 27.6 & 12.2 & 24.8 & 57.4   & 4.2/118/681 \\
% Setup 5 (NYT)                  & 27.2 & 11.8 & 24.4 & 56.9   & 4.1/119/678 \\
% Setup 1 (CNNDM)  & 53.1 & 41.7 & 49.6 & 75.4 & 3.4/106/570 \\
% Setup 2  (CNNDM) & 58.7 & 48.2 & 55.2 & 79.3 & 3.1/95/514  \\
% Setup 3 (CNNDM)  & 28.0 & 10.9 & 24.8 & 56.8 & 3.5/72/397  \\
% Setup 4 (CNNDM)  & 29.7 & 12.4 & 26.2 & 57.8 & 3.4/74/410  \\
% Setup 5 (CNNDM)  & 30.2 & 13.1 & 26.8 & 55.5 & 3.4/78/428 
% \end{tabular}
% \caption{Two annotation - GSUM}
% \end{table*}
